# Supplementary material for: Stackelberg Attacks on Auctions and Blockchain Transaction Fee Mechanisms
Source: arXiv:2305.02178 source file (2023-05-03)
Supplement: Supplementary file 1 [file 4_appendix.tex]

\begin{theorem}[Hall-Andersen, Schwartzbach, \cite{smart_contracts}]\label{thm:pspace}
    Computing the SPE in games with smart contracts is \PSPACE-hard in general, even for games of perfect information. However, there is a quadratic-time algorithm that computes the SPE in two-contract games of perfect information. 
\end{theorem}

We restate the algorithm, simplified to work only on two-player games, for self-containment. Let player 1 have the first contract, and player 2 the the second. Let $A,B \subseteq \mathbb{R}$ and define,
$$
    \textsf{threaten}(A,B) = \{x \in A \mid \exists y \in B. \, y_2 < x_2\}.
$$
as the set of nodes from $A$ that player 1 can threaten player 2 into accepting, using threats from $B$. The algorithm, which we will call Algorithm 1, computes the set of nodes that are inducible by a contract for the first player (the inducible region \cite{inducibleregion}) and selects the node that maximizes their utility. For simplicity, assume $G$ is a bifurcating tree. The algorithm recursively computes the nodes that player 1 can induce in the left and right subtrees and combines them at each branch.

\begin{algorithm}\hspace{-1.125mm}\textsc{\textup{(Hall-Andersen, Schwartzbach, \cite{smart_contracts})}}.\\[2mm]$\textsf{InducibleRegion}(G):$
\begin{enumerate}
    \item[1.] If $G$ is a leaf $\ell$, stop and return $\{\ell\}$.
    \item[2.] If $G$ is a node owned by $i$, with children $G^L$ and $G^R$:
    \begin{enumerate}
        \item[] $I^L \gets \textsf{InducibleRegion}(G^L)$.
        \item[] $I^R \gets \textsf{InducibleRegion}(G^R)$.
        \item[] If $i=1$:
        \begin{enumerate}
            \item[] return $I^L \cup I^R \cup \textsf{threaten}(L, I^L \cup I^R)$.
        \end{enumerate}
        \item[] If $i=2$:
        \begin{enumerate}
            \item[] return $\textsf{threaten}(I^R, I^L)\cup\textsf{threaten}(I^L,I^R)$.
        \end{enumerate}
    \end{enumerate}
\end{enumerate}
\end{algorithm}
In practice, running a smart contract requires submitting multiple queries to the blockchain which requires work by the miners and is not free. For the purposes of this work, however, we regard transaction fees as negligible such that we may disregard them entirely. This holds true if the valuations are large compared to the transaction fees.

\begin{thm}\label{thm:downward_transitive}
  If a game $G$ is side contract 2-resilient, it is also side contract 1-resilient.
\end{thm}
\begin{proof}
We start by showing that omitting the second contract, wlog. that of player 2, from a 2-resilient game still yields the same equilibrium. If the game in which only player 1 has a contract had a different outcome, there must be at least one node in $G$ for which the corresponding set $I$ is different. Let $G^*$ be the lowest such node and observe that by definition this cannot be a leaf. Suppose $G^*$ were owned by 2; given that 2 has no contract, 2 will pick the local SPE child from $I^L \cup I^R$. It is easy to see that $\textsf{threaten}(I^L,I^R)\subseteq I^L\subseteq L^L$, where $L^L$ denotes the leaves of the left subtree, and analogously so on the right. Since this game is 2-resilient, the optimal choice for 2 will correspond to both the universal SPE and the 2-contract choice and therefore also the local SPE. Given that the $I^L$ and $I^R$ are the same, because $G^*$ is the lowest deviant node, we have a contradiction. If instead, $G^*$ is owned by 1, $I^L\cup I^R$ will be the same as in the 2-contract case since $I^L$ and $I^R$ are the same. Since $I^L$ and $I^R$ are the same by assumption, there are no new threats to make  Thus $I$ is unchanged and we again have a contradiction. Thus removing the second contract in a 2-resilient game will not change the equilibrium. Applying this to both orders of contract arrangement gives the desired result. 
\end{proof}
